# Supplementary material for: Understanding Reinforcement Learning-Based Fine-Tuning of Diffusion Models: A Tutorial and Review
Source: arXiv:2407.13734 source file (2024-07-18)
Supplement: Supplementary file 1 [file main_appendix.tex]

\section{Additional Related Works}\label{sec:additional}

\paragraph{Conservative approaches in offline RL/offline contextual bandits. }

\paragraph{Overoptimization in LLMs.}

\section{Summary of Planning Algorithms}\label{sec:sum_planning}

In this section, we summarize algorithms that can solve  Equation~\eqref{eq:key_plnanning}. 

\subsection{Direct Back Propagation}

\begin{algorithm}[!t]
\caption{Direct Back Propagation }\label{alg:main}
\begin{algorithmic}[1]
     \STATE {\bf Require}: Set a diffusion-model $\{\Ncal(\rho(t,x_{t};\theta),\sigma^2_t); \theta \in \Theta\}_{t=T+1}^1$, pre-trained model $\{\Ncal(\rho(t,x_{t};\theta_{\pre}),\sigma^2_t)\}_{t=T+1}^1$, batch size $m$, a parameter $\alpha \in \RR^+$. 
     \STATE {\bf Initialize}: $\theta_1 = \theta_{\pre}$
     \FOR{$s \in [1,\cdots,S]$}
      \STATE Set $\theta = \theta_s$. 
      \STATE Collect $m$ samples $\{x^{(i)}_t(\theta) \}_{t=T+1}^0$ from a current diffusion model (i.e., generating by sequentially running polices $\{\Ncal(\rho(t,x_{t};\theta),\sigma^2_t)\}_{t=T+1}^1$ from $t=T+1$ to $t=1$) 
      \STATE Update $\theta_s$ to $\theta_{s+1}$ by adding the gradient of the following loss $L(\theta)$ with respect to $\theta$ at $\theta_s$: 
      \begin{align}\label{eq:key}
   & L(\theta) = \frac{1}{m} \sum_{i=1}^m  \left[\hat r(x^{(i)}_0(\theta) ) - \hat g(x^{(i)}_0(\theta) ) -  \alpha     \sum_{t=T+1}^1 \frac{\|\rho(x^{(i)}_t(\theta),t;\theta)-\rho(x^{(i)}_t(\theta),t; \theta_{\pre}) \|^2 }{2\sigma^2(t) } \right ] . 
      \end{align}  
      \ENDFOR
  \STATE {\bf Output}: Policy $\{p_t(\theta_S) \}_{t=T+1}^1$   
\end{algorithmic}
\end{algorithm}

\subsection{Proximal Policy Gradient (PPO) }

\citet{fan2023dpok,clark2023directly} propose using PPO algorithms in the online setting. We can readily adapt their approach to our offline setting. One potential advantage of using PPO in an online context is the ability to utilize reward queries directly without the need to train differentiable reward models $\hat r:\Xcal \to \RR$. However, in our offline scenario, as we train the differentiable reward model regardless, we cannot leverage this advantage. Therefore, we still suggest that users employ direct backpropagation.

\subsection{Value Weighted Regression}  

From \pref{thm:key2}, recall the form of the optimal policy $\hat p_t(x_{t-1}|x_t)$:
\begin{align*}
     \frac{\exp(v_{t-1}(x_{t-1})/\alpha)\hat p^{\pre}_{t}(x_{t-1}|x_{t})}{C}
\end{align*}
Now, let's consider the KL divergence:
\begin{align*}
    \EE_{x_t \sim u_t }[\KL (\hat{p}_t(\cdot|x_t) \|  p_t(\cdot|x_t))  ] 
\end{align*}
where $u_t \in \Delta(\Xcal)$ is a roll-in distribution that covers the entire space $\Xcal$. Then, since 
\begin{align*}
   \hat p_t =   \argmin_{p_t:\Xcal \to \Delta(\Xcal) } \EE_{x_t \sim u_t }[\KL (\hat{p}_t(\cdot|x_t) \|  p_t(\cdot|x_t))  ] 
\end{align*}
we obtain the following. 

\begin{lemma}[Value weighted MLE]\label{lem:value}
When $\Pi_t =[\Xcal \to \Delta(\Xcal)] $, the policy $\hat p_t$ is given by  
    \begin{align*}
 \hat p_t(\cdot|\cdot) = \argmin_{p_t \in \Pi_t} \EE_{x_{t-1}\sim p^{\pre}_{t-1}(x_{t}),x_t\sim u_t }\left[\exp\left( \frac{v_{t-1}(x_{t-1})}{\alpha}\right) \log p_t(x_{t-1}|x_t) \right ], 
\end{align*}
where $v_{t-1}(\cdot)$ is the optimal soft value function. 
\end{lemma}

This lemma demonstrates that if we know $v_{t-1}$, we can estimate $\hat p_t$ by conducting weighted maximum likelihood estimation (MLE). Although we discuss how to estimate $v_{t-1}(\cdot)$ later, we can actually perform weighted MLE without directly estimating it. To see this, let's utilize the following lemma:

\begin{lemma}[Characterization of soft optimal value functions]\label{lem:characterization}
    \begin{align*}
   \exp\left(\frac{v_t(x_t)}{\alpha} \right) = \EE_{ \{p^{\pre}_t\} }\left[\exp\left(\frac{\hat r(x_0)-\hat g(x_0)}{\alpha} \right )|x_t \right ], 
\end{align*}
where the expectation is taken with respect to the distribution induced by $ \{p^{\pre}_t\}$. 
\end{lemma}
\begin{proof}
This is obtained by recursively using the soft-Bellman equation  \eqref{eq:soft}: 
\begin{align}
 \exp\left (\frac{ v_{t}(x_{t})}{\alpha}\right )& = \int \exp\left (\frac{ v_{t-1}(x_{t-1})}{\alpha}\right)p^{\pre}_{t}(x_{t-1} \mid x_{t}) d x_{t-1}.  
\end{align}
\end{proof}

Now, by combining \pref{lem:value} and \pref{lem:characterization}, we obtain:
    \begin{align*}
 \argmin_{p_t \in \Pi_t} \EE_{x_{t-1}\sim p^{\pre}_{t-1}(x_{t}),x_t\sim u_t }\left[\exp\left(\frac{\hat r(x_0)-\hat g(x_0)}{\alpha}\right) \log p_t(x_{t-1}|x_t) \right ], 
\end{align*}
Then, using a Gaussian policy class with the mean parameterized by neural networks as $\Pi_t$ and replacing the expectation with empirical approximation, the entire algorithm is described in Algorithm~\ref{alg:weightedMLE}.

\begin{remark}
Similar approaches have been employed in \citet{fan2023dpok} (+ XXX). However, our formal characterization in soft entropy-regularized MDPs seems to be novel.
\end{remark}

\subsection{Value Weighted Sampling}

\begin{algorithm}[!t]
\caption{(Monte Carlo) Value weighed regression}\label{alg:weightedMLE}
\begin{algorithmic}[1]
     \STATE {\bf Require}:  Exploratory roll-in policies $\{u_{t}(x_{t-1}|x_t)\}_t$, pre-trained policies $\{p^{\pre}_{t}(x_{t-1}|x_t)\}_t$. 
    \FOR{$t \in [T+1,\cdots,1]$}
      \STATE Collect $m$ samples $\{x^{(i,t)}_0\}_{i=1}^m$ from a policy $u_{T+1},\cdots,u_{t},p^{\pre}_{t},\cdots,p^{\pre}_{1} $.  
     \ENDFOR
      \STATE Define $\hat \theta$ by solving the below:  
      \begin{align}\label{eq:key}
 \hat \theta = \argmin_{\theta}\sum_{t=T+1}^1 \sum_{i=1}^m  \left[\exp \left (\frac{(\hat r-\hat g)(x^{(i,t)}_0)}{\alpha} \right)\|x^{(i,t)}_{t-1} -\rho(x^{(i,t)}_t,t;\theta) \|^2_2   \right]. 
      \end{align}  
  \STATE {\bf Output}: A policy $\{\Ncal(\rho(x_t,t;\hat \theta),\sigma^2_t )  \}_t$ 
\end{algorithmic}
\end{algorithm}

\begin{algorithm}[!t]
\caption{Value weighted sampling}\label{alg:value_sampling}
\begin{algorithmic}[1]

 \STATE {\bf Require}:  Pre-trained policies $\{p^{\pre}_{t}(x_{t-1}|x_t)\}_t = \{ \Ncal(\rho(x_t,t; \theta_{\pre}),\sigma^2_t)\}_t $. 
    \FOR{$t \in [T+1,\cdots,1]$}
      \STATE Estimate $v_t:\Xcal \to \RR$ using value-weighted regression in \pref{lem:characterization}  and denote it by $\hat v_t$ 
      \STATE Set 
     \begin{align*}
        \rho(x_t,t; \theta^{\star}):= \frac{\sigma^2_t \nabla_x \hat v_t(x_t)}{\alpha}  + \rho(x_t,t; \theta_{\pre}). 
\end{align*}
\ENDFOR 
  \STATE {\bf Output}: $\{\Ncal(\rho(x_t,x; \theta^{\star}),\sigma^2_t)\}$
\end{algorithmic}
\end{algorithm}

So far, we have explored methods to fine-tune pre-trained diffusion models. Now, we delve into an alternative approach that does not involve explicit fine-tuning of diffusion models.

Consider a Gaussian policy $x_{t-1}\sim \Ncal(\rho(x_t,t;\theta),\sigma^2_t)$. Suppose there exists $\theta^{\star}$ that $\Ncal(\rho(x_t,t;\theta^{\star}),\sigma^2_t) = \hat p_t(\cdot|x_t).$ In such a scenario, taking the gradient with respect to $x_{t-1}$ on both sides yields:
\begin{align*}
    \frac{x_{t-1}- \rho(x_t, t; \theta^{\star})}{\sigma^2_t} = \nabla_x v_{t-1}(x_{t-1} ) +  \frac{x_{t-1}- \rho(x_t, t; \theta_{\pre})}{\sigma^2_t} 
\end{align*}
Rearranging the terms, we get:
\begin{align*}
    \rho(x_t, t; \theta^{\star}) = \frac{\sigma^2_t \nabla_x v_{t-1}(x_{t-1})}{\alpha} + \rho(x_t, t; \theta_{\pre}). 
\end{align*}
Motivated by the above, and noting $\nabla_x v_{t-1}(x_{t-1}) \approx \nabla_x v_{t-1}(x_{t})$, we can approximate:
\begin{align*}
    \rho(x_t, t; \theta^{\star}) \approx \frac{\sigma^2_t \nabla_x v_{t-1}(x_{t-1})}{\alpha} + \rho(x_t, t; \theta_{\pre}). 
\end{align*}

Using the above, the whole algorithm is outlined in Algorithm~\ref{alg:value_sampling}. Note that in this algorithm, we require a form of $v_t(\cdot)$ to compute gradients. This can be readily estimated through regression using the characterization described in Lemma~\ref{lem:characterization}, and by noting:
\begin{align}\label{eq:estimate_value}
     v_t = \argmin_{h:\Xcal \to \RR } \EE_{\{p^{\pre}_t\}} \left[\left \{ \exp\left(\frac{h(x_t)}{\alpha} \right) - \exp\left(\frac{\hat r(x_0)-\hat g(x_0)}{\alpha} \right ) \right \}^2  \right ] 
\end{align}
where the expectation is taken w.r.t. distribution induced by pre-trained models.

\subsection{Soft Q-learning}

We have elucidated that leveraging Lemma~\ref{lem:characterization}, we can estimate optimal soft value functions $v_t(\cdot)$ based on Equation~\eqref{eq:estimate_value}. Similarly, we can use soft-Q-learning to estimate soft-value functions $v_t(\cdot)$.

Recalling the soft Bellman equations:
\begin{align*} 
\exp \left  (\frac{ v_{t}(x_{t})}{\alpha} \right )=  \int \exp\left (\frac{ v_{t-1}(x_{t-1})}{\alpha}\right)p^{\pre}_{t}(x_{t-1} \mid x_{t}) d x_{t-1}. 
\end{align*}
Taking the logarithm:
\begin{align*} 
 v_{t}(x_{t}) = \alpha \log \int \exp\left (\frac{ v_{t-1}(x_{t-1})}{\alpha}\right)p^{\pre}_{t}(x_{t-1} \mid x_{t}) d x_{t-1}. 
\end{align*}
Hence: 
\begin{align*}
     v_t = \argmin_{h:\Xcal \to \RR}\EE_{x_t\sim u_t} \left[\left \{\frac{h(x_t)}{\alpha} -\log \int \exp\left( \frac{v_{t-1}(x_{t-1})}{\alpha} \right)p_{\pre}(x_{t-1}|x_t) d x_{t-1}  \right \}^2   \right ]
\end{align*}
where $u_t \in \Delta(\mathcal{X})$ is any roll-in distribution that covers the entire space $\mathcal{X}$. Then, the optimal policy is obtained by plugging the estimated soft optimal value valuation into value-weighted regression in Algorithm~\ref{alg:weightedMLE} or value-weighted sampling in Algorithm~\ref{alg:value_sampling}. This procedure is summarized in Algorithm~\ref{alg:soft_q_learning}.

\begin{algorithm}[!t]
\caption{Soft-Q-learning}\label{alg:soft_q_learning}
\begin{algorithmic}[1]
 \STATE {\bf Require}: Exploratory roll-in policies $\{u_{t}(x_{t-1}|x_t)\}_t$, pre-trained policies $\{p^{\pre}_{t}(x_{t-1}|x_t)\}_t$, learning rate $\gamma_s$. 
 \STATE Set a model $\{v_t(\cdot;\theta)\}$ to learn optimal soft-value functions.  
      \FOR{$s=\{0,\cdots,S\}$}
      \STATE Set $\phi_{\mathrm{old}} = \phi $
      \STATE Set $v_0 = \hat r-\hat g$
      {\small 
     \begin{align*}
    \phi  \leftarrow \phi-\gamma_s \nabla_{\phi} \sum_{t=T+1}^1  \hat \EE_{x_t \sim u_t}\left[\left \{\frac{v_t(x_t;\phi)}{\alpha} -\log \hat \EE_{x_{t-1} \sim p_{\pre}(\cdot|x_t)}\left[ \exp\left( \frac{v_{t-1}(x_{t-1};\phi_{\mathrm{old}})}{\alpha} \right)|x_t\right]  \right \}^2   
    \right ] 
     \end{align*}
     } 
     where $\hat \EE[\cdot]$ is an empirical approximation. 
   \ENDFOR 
  \STATE {\bf Output}: $\{v_t(x;\phi_S)\}_t$
\end{algorithmic}
\end{algorithm}

\subsection{Training with Detailed Balance Loss (Standard Training Algorithms in Gflownets)}

\begin{algorithm}[!t]
\caption{Training with detailed balance loss}\label{alg:detailed_balance_loss}
\begin{algorithmic}[1]
 \STATE {\bf Require}: Exploratory roll-in policies $\{u_{t}(x_{t-1}|x_t)\}_t$, pre-trained policies $\{p^{\pre}_{t}(x_{t-1}|x_t)\}_t$, learning rate $\gamma_s$. 
  \STATE Set a model $\{v_t(\cdot;\theta)\}$ to learn optimal soft value function, and a model $\{ p_t(\cdot|\cdot ;\psi)\} $ to learn optimal polices. 
      \FOR{$s=\{0,\cdots,S\}$}
      \STATE Set $\phi_{\mathrm{old}} = \phi,  \psi_{\mathrm{old}} = \psi$
      \STATE Set $v_0 = \hat r-\hat g$ 
      {\small 
     \begin{align*}
    \phi  \leftarrow \phi -\gamma_s \nabla_{\phi} \sum_{t=T+1}^1  \hat \EE_{x_t \sim u_t}\left[\left \{\frac{v_t(x_t;\phi)}{\alpha} + \log p_t(x_{t-1}|x_t;\psi) -  \frac{v_{t-1}(x_{t-1};\phi_{\mathrm{old}})}{\alpha} + \log p^{\pre}_t(x_{t-1}|x_t)  \right \}^2    
    \right ] , \\ 
     \psi  \leftarrow \psi -\gamma_s \nabla_{\psi} \sum_{t=T+1}^1  \hat \EE_{x_t \sim u_t}\left[\left \{\frac{v_t(x_t;\phi)}{\alpha} + \log p_t(x_{t-1}|x_t;\psi) - \frac{v_{t-1}(x_{t-1};\phi_{\mathrm{old}})}{\alpha}  + \log p^{\pre}_t(x_{t-1}|x_t)  \right \}^2    
    \right ], 
     \end{align*}
     } 
     where $\hat \EE[\cdot]$ is an empirical approximation. 
   \ENDFOR 
  \STATE {\bf Output}: $\{p_t(x_{t-1}|x_t;\psi_S) \}_t$
\end{algorithmic}
\end{algorithm}

In the literature on Gflownets \citep{bengio2023gflownet}, it seems they suggest employing a variant of soft-Q-learning more tailored to our context, as elucidated in \citet{mohammadpour2023maximum,tiapkin2023generative,deleu2024discrete}.
Now, from Theorem~\ref{thm:key2}, we derive:
\begin{align*}
     \underbrace{\frac{1}{C}\exp\left (\frac{ v_{t}(x_{t})}{\alpha} \right )p^{\pre}_t(x_t) }_{\text{Marginal distribution at t}}\times   \underbrace{\hat p_t(x_{t-1}|x_{t})}_{\text{optimal policy}} = \underbrace{\frac{1}{C} \exp\left (\frac{ v_{t-1}(x_{t-1})}{\alpha} \right ) p^{\pre}_{t-1}(x_{t-1})}_{\text{Marginal distribution at t-1} }\times  \underbrace{p^{\pre}_{t-1}(x_{t}|x_{t-1})}_{\text{Posterior distribution}}
\end{align*}
Rearranging yields:
\begin{align*}
    \frac{1}{C}\exp\left (\frac{ v_{t}(x_{t})}{\alpha} \right )\times \hat p_t(x_{t-1}|x_{t}) = \frac{1}{C} \exp\left (\frac{ v_{t-1}(x_{t-1})}{\alpha} \right ) \times  p^{\pre}_t(x_{t-1}|x_{t})
\end{align*}
Taking the logarithm, we obtain: 
\begin{align}\label{eq:detailed}
    \left(\frac{ v_{t}(x_{t})}{\alpha}\right) + \log \hat p_t(x_{t-1}|x_{t}) =  \left( \frac{ v_{t-1}(x_{t-1})}{\alpha}\right) + \log  p^{\pre}_t(x_{t-1}|x_{t})
\end{align}
Thus, initializing $v_{0}=\hat r-\hat g$, we obtain the recursive equation: 
{\small 
\begin{align}\label{eq:loss_gflownets}
    (v_t,\hat p_t) = \argmin_{g^{(1)}:\Xcal \to \RR, g^{(2)}:\Xcal \to \Delta(\Xcal)}\EE_{x_t \sim u_t}\left[  \left\{  \frac{ g^{(1)}(x_{t})}{\alpha}  + \log g^{(2)}(x_{t-1}|x_{t})-  \frac{ v_{t-1}(x_{t-1})}{\alpha} -  \log  p^{\pre}_t(x_{t-1}|x_{t})\right\}^2 \right ]
\end{align}
} 
where $u_t \in \Delta(\mathcal{X})$ is any exploratory roll-in distribution. This loss is often referred to as a detailed balance loss \citep{bengio2023gflownet}. Based on this rationale, we outline the entire algorithm in Algorithm~\ref{alg:detailed_balance_loss}.

\begin{remark}
In standard literature on Gflownets, $p^{\pre}_t(x_{t-1}|x_t)$ is typically substituted with a backward policy $p^{b}_t(x_{t}|x_{t-1})$ in \eqref{eq:detailed} and \eqref{eq:loss_gflownets}.
\end{remark}

\section{All Proofs}

\subsection{Proof of Theorem~\ref{thm:key}}\label{thm:key_proof}

Here, we actually prove a stronger statement as follows. 

\begin{theorem}[Marginal and Posterior distributions]\label{thm:key2}
Let $\hat p_t(x_t)$ and $\hat p^b_{t}(x_{t}| x_{t-1})$ be  marginal distributions at $t$ or posterior distributions of $x_{t}$ given $x_{t-1}$, respectively, induced by optimal policies $\{\hat p_t\}_{T+1}^1$. Then, 
\begin{align*}
    \hat p_t(x_t) =  \exp(v_{t}(x_{t})/\alpha)\hat p^{\pre}_{t}(x_{t})/C,\quad \hat p^b_t(x_{t}|x_{t-1}) = \hat p^{\pre}_t(x_{t}|x_{t-1}). 
\end{align*}
\end{theorem}  

 To simplify the notation, we let $r(x) =  \hat r(x)- \hat g(x)$. 

 As a first step, by using induction, we aim to obtain an analytical form of the optimal policy $\{\hat p_t\}$. First, we define the soft-optimal value function as follows: 
\begin{align*}
v_{t-1}(x_{t-1})  = \EE_{\{\hat p_t\} }\left[f(x_0) - \beta \sum_{k=t-1}^1 \KL(\hat p_k(\cdot|x_k) \|p^{\pre}_k(\cdot|x_k)) | x_{t-1} \right]. 
\end{align*}
Then, by induction, we have 
\begin{align*}
 \hat p_t(x_{t-1}|x_t) =\argmax_{ p_t \in \Delta(\Xcal) } \EE_{\{\hat p_t\} }\left [ v_{t-1}(x_{t-1}) - \beta \KL(p_t(\cdot|x_t) \|p^{\pre}_t(\cdot|x_t)) |x_t \right].   
\end{align*}
With some algebra, we obtain 
\begin{align*}
\hat p_t(x_{t-1}|x_t) \propto \exp\left(\frac{v_{t-1}(x_{t-1}) }{\beta} \right)  p^{\pre}_t(x_{t-1}|x_t) . 
\end{align*}
Here, noting 
\begin{align*}
 v_t(x_t) =\max_{p_t \in \Delta(\Xcal) } \EE_{\{\hat p_t\} }[ v_{t-1}(x_{t-1}) - \beta \KL(p_t(\cdot|x_t) \|p^{\pre}_t(\cdot|x_t)) |x_t ],
\end{align*}
we get the soft Bellman equation:
\begin{align*}
  \exp\left(\frac{v_{t}(x_{t}) }{\beta} \right)  = \int \exp\left(\frac{v_{t-1}(x_{t-1}) }{ \beta} \right)  p^{\pre}_t(x_{t-1}|x_t) \mathrm{d}x_{t-1}. 
\end{align*}
Therefore, we actually have 
\begin{align}\label{eq:soft_formulation}
 \hat p_t(x_{t-1}|x_t)=\frac{ \exp\left(\frac{v_{t-1}(x_{t-1}) }{\beta} \right) p^{\pre}_t(x_{t-1}|x_t)}{  \exp\left(\frac{v_{t}(x_{t}) }{\beta} \right)   } .
\end{align}

Finally, we calculate the marginal distribution 
\begin{align*}
    \hat p_t(x_t):=\int \left\{ \prod_{s=T+1}^t \hat p_{s}(x_{s-1}|x_s) \right\} dx_{t+1:T+1}. 
\end{align*}
Now, by using induction, we aim to prove 
\begin{align*}
    \hat p_{t}(x_{t})=  \exp\left(\frac{v_{t}(x_{t}) }{\beta} \right)p^{\pre}_{t}(x_{t}). 
\end{align*}
Indeed, when $t=T+1$, this hold as follows: 
\begin{align*}
    \hat p_{T+1}(x_{T+1}) = \frac{1}{C}  \exp\left(\frac{v_{T}(x_{T+1}) }{ \beta} \right)p^{\pre}_{T+1}(x_{T+1}). 
\end{align*}
Now, suppose the above holds at $t$. Then, this also holds for $t-1$: 
\begin{align*}
      \hat p_{t-1}(x_{t-1})& =\int  \hat p_t(x_{t-1}|x_t)   \hat p_{t}(x_{t})\mathrm{d}x_t  \\
      &=\int \exp\left(\frac{v_{t-1}(x_{t-1}) }{\beta} \right) \{ p^{\pre}_t(x_{t-1}|x_t) \} p^{\pre}_{t}(x_{t}) \mathrm{d}x_t  \tag{Use Equation~\ref{eq:soft_formulation}}  \\
      &= \exp\left(\frac{v_{t-1}(x_{t-1}) }{\beta} \right)p^{\pre}_{t-1}(x_{t-1}). 
\end{align*}
By invoking the above when $t=0$, the statement is concluded.

\subsection{Proof of Theorem~\ref{thm:regret} }

In this section, we suppose the support of $\pi$ is included in that of $p_{\un}$. If not, the soft value takes $\infty$. In the following, we condition on the event where 
\begin{align*}
  \forall x\in \Xcal_{\pre};  |r(x) - \hat r(x)| \le g(x). 
\end{align*}
holds. 

First, we define 
\begin{align*}
    \hat J_{\alpha}(\pi) &:= \EE_{x \sim \pi}[ \hat r(x)-\hat g(x) ] -\alpha \mathrm{KL}(\pi \| p_{\un}),\quad J_{\alpha}(\pi):= \EE_{x \sim \pi}[ r(x)] -\alpha \mathrm{KL}(\pi \| p_{\un}). 
\end{align*}
We note that, $\hat{\pi}_\alpha$ maximizes $\hat{J}_\alpha(\pi)$. Therefore, we have 
\begin{align*}
       J_{\alpha}(\pi)- J_{\alpha}(\hat \pi_\alpha)&= J_{\alpha}(\pi)-  \hat J_{\alpha}(\pi)+ \hat J_{\alpha}(\pi)-  \hat J_{\alpha}(\hat \pi_\alpha)+    \hat J_{\alpha}(\hat \pi_\alpha)- J_{\alpha}(\hat \pi_\alpha)\\
    &\leq J_{\alpha}(\pi)-  \hat J_{\alpha}(\pi) +    \hat J_{\alpha}(\hat \pi_\alpha)- J_{\alpha}(\hat \pi_\alpha) \tag{Definition of $\hat \pi_\alpha$} \\
    &\stackrel{\text{(i)}}{\leq} J_{\alpha}(\pi)-  \hat J_{\alpha}(\pi). \tag{Pessimism}
\end{align*}
Here, in the step (i), we use 
\begin{align*}
  \forall x\in \Xcal_{\pre};  |r(x) - \hat r(x)| \le g(x). 
\end{align*}
Then, 
\begin{align*}
    J_{\alpha}(\pi)- J_{\alpha}(\hat \pi_\alpha)   & \leq J_\alpha(\pi) - \hat{J}_\alpha(\pi)  \leq 2\EE_{x\sim \pi} [\hat g(x)] \\
    & \leq 2 \left\|\frac{\pi}{p_{\pre} }\right\|_{\infty}\EE_{x\sim p_{\pre}}[\hat g(x)] \tag{Importance sampling}. 
\end{align*}
Hence, the statement is concluded.

\section{Theoretical Guarantees with Gaussian Processes} \label{sec:GPs}

In this section, we explain the theoretical guarantee when using Gaussian processes.   

\subsection{Preparation}

We introduce the notation to state our guarantee. For details, see \citet[Appendix B]{srinivas2009gaussian}, \citet[Chapter 6.2]{uehara2021pessimistic}, \citet[Chapter C.3]{chang2021mitigating}. 

For simplicity, we first suppose the following. 
\begin{assum}
   The space $\Xcal$ is compact, and $\forall x \in \Xcal; k(x,x)\leq 1$. 
\end{assum}

We introduce the following definition. Regarding details, refer to \citet[Chapter 12]{wainwright2019high}. 
\begin{definition}
   Let $\Hcal_k$ be the RKHS with the kernel $k(\cdot,\cdot)$. We denote the associated norm and inner product by $\|\cdot\|_k,\langle \cdot,\rangle_k$, respectively. We introduce analogous notations for 
   \begin{align*}
        \hat k(x,x')= k(x,x')-\kb_i(x)^{\top}\{ \Kb_i+\lambda I \}^{-1}  \kb_i(x'). 
   \end{align*}
   and denote the norm and inner product by $\|\cdot\|_{\hat k},\langle \cdot,\rangle_{\hat k}$. 
\end{definition}
Note as explained in  \citet[Appendix B]{srinivas2009gaussian} and \citet[Chapter C.3]{chang2021mitigating}, actually, we have $\Hcal_k =\Hcal_{\hat k}$.  

In this section, we suppose the model is well-specified. 
\begin{assum}
   $ y = r(x) + \epsilon$ where $\epsilon\sim \Ncal(0,I)$ where $r$ belongs to an RKHS in $\Hcal_k$.  
\end{assum}

In the following, We use the feature mapping associated with an RKHS $\Hcal_k$. To define this, from Mercer's theorem, note we can ensure the existence of orthonormal eigenfunctions and eigenvalues $\{\psi_i,\mu_i\}$ such that 
\begin{align*}
    k(\cdot,\diamond)=\sum_{i=1}^{\infty} \mu_i \psi_i(\cdot ) \psi_i(\diamond), \begin{cases} \int\psi_i(x)\psi_i(x)p_{\spp}(x)dx =1 \\ \int\psi_i(x)\psi_j(x)p_{\spp}(x)dx =0 (i\neq j)   \end{cases}. 
\end{align*}
Then, we define the feature mapping: 
\begin{definition}[Feature mapping]
    \begin{align*}
        \phi(x):=[\sqrt{\mu_1}\psi_1(x), \sqrt{\mu_1}\psi_1(x),\cdots]^{\top}. 
    \end{align*}
\end{definition}
Assuming eigenvalues are in non-increasing order, we cam also define the effective dimension following \citet[Appendix B]{srinivas2009gaussian}, \citet[Chapter 6.2]{uehara2021pessimistic}, \citet[Chapter C.3]{chang2021mitigating}:  
\begin{definition}[Effective dimension]
\begin{align*}
    d' = \min_{j} \left \{j \in \mathbb{N}: j \geq  n\sum_{k=j}^{\infty}\mu_k\right \}. 
\end{align*}
\end{definition}
The effective dimension is commonly used and calculated in many kernels (XXX). In finite-dimensional linear kernels $\{x\mapsto a^{\top}\phi(x):a\in \RR^d \}$ such that $k(x,z) =\phi^{\top}(x)\phi(z)$, letting 
$d'\coloneqq \rank(\EE_{x \sim p_{\spp} }[\phi(x)\phi(x)]$), we have 
\begin{align*}
     d' \leq \tilde d \leq d 
\end{align*}
because there exists $\mu_{\tilde d+1}=0,\mu_{\tilde d+2} =0,\cdots$.

\subsection{Calibrated oracle}

We use a result in \citep{srinivas2009gaussian}. 
Let 
\begin{align*}
    C(\delta) = c_1 \sqrt{1+ \log^3(n/\delta) \Ical_{n}},\quad \Ical_n = \log(\det(I+\Kb)). 
\end{align*}
Then, with probability $1-\delta$, 
\begin{align*}
    \hat r(x)-r(x) & = \langle \hat r(\cdot)-r(\cdot), \hat k(\cdot,x)\rangle_{\hat k}  \tag{Reprocuding property } \\ 
    & \leq   \|\hat r(\cdot)-r(\cdot)\|_{\hat k} \times \|\hat k(\cdot,x)\|_{\hat k}  \tag{CS inequality } \\
    &\leq \|\hat r(\cdot)-r(\cdot)\|_{\hat k}\sqrt{\hat k(x,x)} \\
    & \leq C(\delta) \hat k(x,x). \tag{Use Theorem 6 in \citep{srinivas2009gaussian}} 
\end{align*}

\subsection{Regret Guarantee}

Recall from the proof of \pref{thm:key2}, 
\begin{align*}
    J_{\alpha}(\pi)- J_{\alpha}(\hat \pi_\alpha) \leq 2\EE_{x\sim \pi} [\hat g(x)]=2C(\delta) \EE_{x\sim \pi} [\sqrt{\hat k(x,x)} ]. 
\end{align*}

Now, first, to upper-bound $\EE_{x\sim \pi} [\sqrt{\hat k(x,x)} ]$, we borrow Theorem 25 in \citep{chang2021mitigating}, which shows 
\begin{align*}
    \EE_{x\sim \pi} [\sqrt{\hat k(x,x)} ]\leq c_1\sqrt{\frac{\tilde C_{\pi}d'\{d' + \log(c_2/\delta) \}}{n} }. 
\end{align*}
where 
\begin{align*}
\tilde C_{\pi}:=\sup_{\kappa:\|\kappa \|_2=1 }\frac{\kappa ^{\top}\EE_{x\sim \pi}[\phi(x) \phi^{\top}(x) ] \kappa}{\kappa ^{\top} \EE_{x\sim p_{\spp}}[\phi(x) \phi^{\top}(x)] \kappa}
\end{align*} 
Next, to upper-bound $C(\delta)$, we borrow Theorem 24 in \citep{chang2021mitigating}, which shows 
\begin{align*}
    \Ical_n \leq c_1\{d' + \log(c_2/\delta)\}d'\log(1+n). 
\end{align*}
The statement in Corollary~\ref{cor:GPS} is immediately concluded.

\section{Additional Details of Experiments} \label{sec:experiments}

\subsection{Biological sequences}

\subsection{Images}
